# Supplementary material for: Learning deep abdominal CT registration through adaptive loss weighting and synthetic data generation
Source: arXiv:2211.15717 ancillary file (2023-02-25)
Supplement: Supplementary file 1 [file supplementary_materials.pdf]

## Supplementary Materials for Train smarter, not harder: learning deep abdominal CT registration on scarce data

Javier Pérez de Frutos<sup>1\*</sup>, André Pedersen<sup>1,2,3</sup>, Egidijus Pelanis<sup>4</sup>, David Bouget<sup>1</sup>, Shanmugapriya Survarachakan<sup>5</sup>, Thomas Langø<sup>1,6</sup>, Ole-Jakob Elle<sup>4</sup>, and Frank Lindseth<sup>5</sup>

<sup>1</sup>*Department of Health Research, SINTEF, Trondheim, Norway*

<sup>2</sup>*Department of Clinical and Molecular Medicine, Norwegian University of Science and University (NTNU), Trondheim, Norway*

<sup>3</sup>*Clinic of Surgery, St. Olavs hospital, Trondheim University Hospital, Trondheim, Norway*

<sup>4</sup>*Intervention Centre, Oslo University Hospital, Oslo, Norway*

<sup>5</sup>*Department of Computer Science, Norwegian University of Science and University (NTNU), Trondheim, Norway*

<sup>6</sup>*Research Department, Future Operating Room, St. Olavs hospital, Trondheim University Hospital, Trondheim, Norway*

\*Corresponding author: Javier Pérez de Frutos, javier.perezdefrutos@sintef.no

## 1 Document description

This document contains supplementary tables and figures that were not part of the main manuscript.

### 1.1 Data description

A total of 28 regions were segmented on the IXI dataset using the MNI 152 space atlas. From these, 24 classes distinguished between left and right sections, which were merged together resulting in a collection of 16 labels. A total of 17 labels, including the background, were used. For more details, see Table S1.

Table S1: Labels used from the MNI 152 space atlas.

|                                        |                                       |
|----------------------------------------|---------------------------------------|
| Parietal grey matter (left and right)  | Fornix (left and right)               |
| Lateral ventricle (left and right)     | Caudate (left and right)              |
| Occipital grey matter (left and right) | Cerebellum (left and right)           |
| Globus pallidus (left and right)       | Thalamus (left and right)             |
| Putamen (left and right)               | Frontal grey matter (left and right)  |
| Subthalamic nucleus (left and right)   | Temporal grey matter (left and right) |
| 3 <sup>rd</sup> ventricle              | Brain stem                            |
| 4 <sup>th</sup> ventricle              | Cerebrospinal fluid                   |
|                                        | Background                            |

## 2 Additional results

### 2.1 Resources impact of the augmentation layer

Figs. S1a and S1b show the GPU usage during one training epoch. The relative increase in time is of 7.7% (ca. 10.5 s). Fig. S1c shows the memory usage on the GPU during one training epoch with and without using the augmentation layer. The increase in memory allocation is of 0.47% (ca. 74 MB / 16 GB).

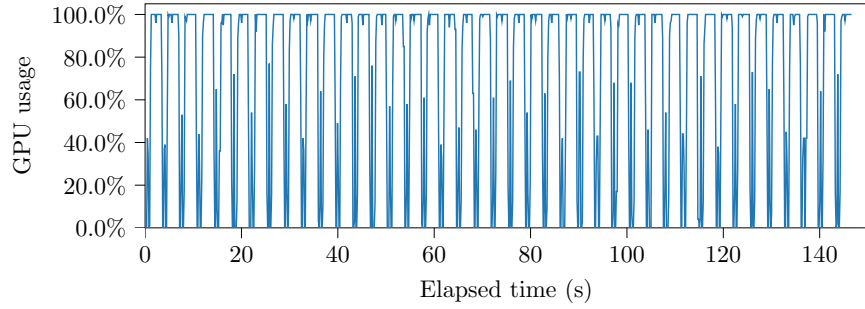

(a) GPU usage with augmentation layer

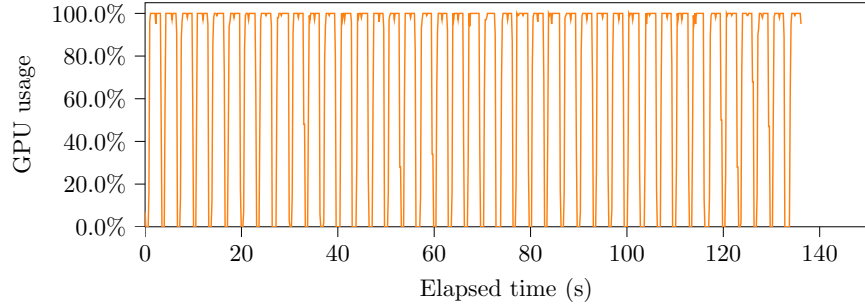

(b) GPU usage without augmentation layer

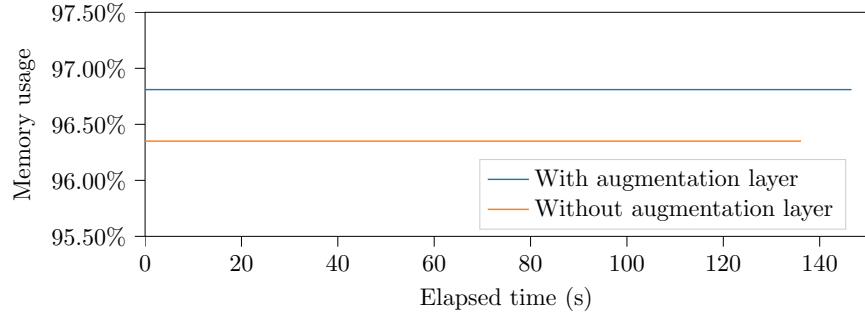

(c) Memory usage with (blue) and without using the augmentation layer (orange)

Figure S1: Impact of the augmentation layer on the GPU resources during one training epoch.

## 2.2 Training curves and runtimes

Figs. S2 - S5 show training and validation losses for the six different training designs described in the main manuscript, for the IXI and OSLO-COMET datasets (see Table 1, Section 2.5). Furthermore, training runtime of 160 epochs is shown as part of the legends of both figures for reference.

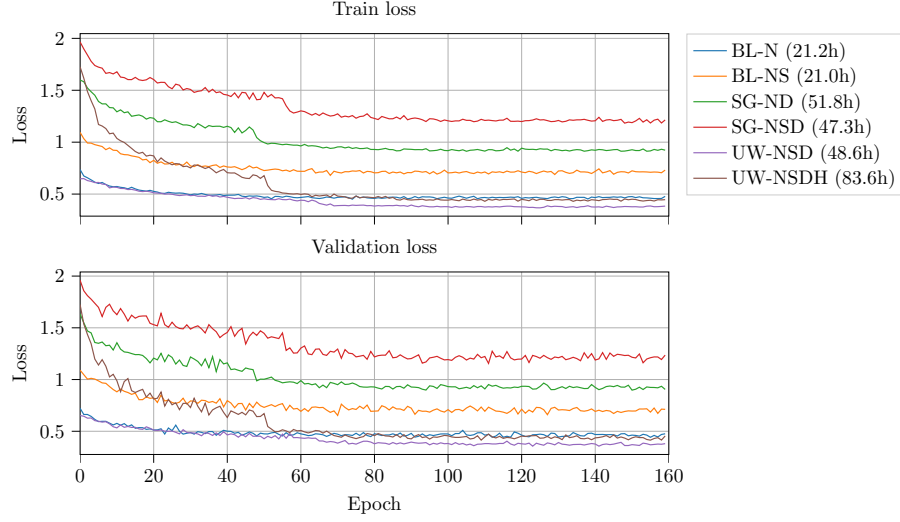

Figure S2: Train and validation loss of the models trained on the IXI dataset.

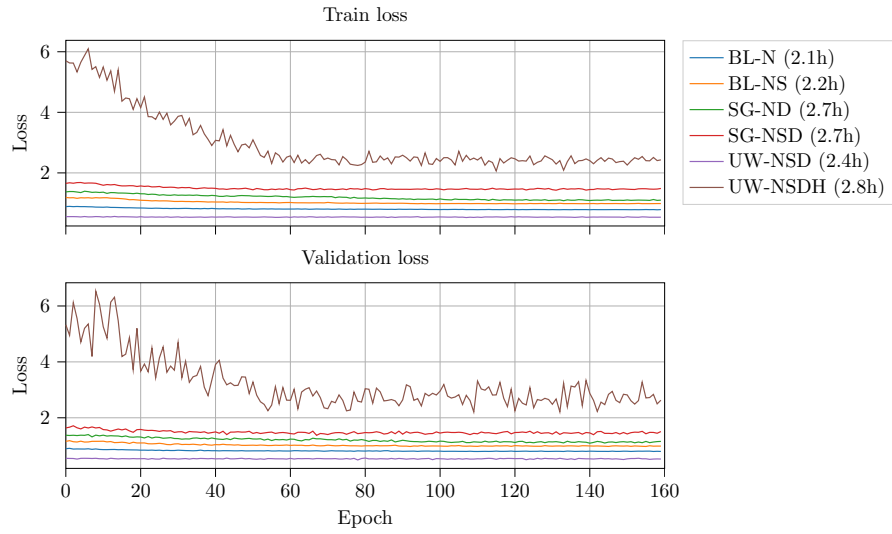

Figure S3: Train and validation loss of the models trained on the OSLO-COMET dataset.

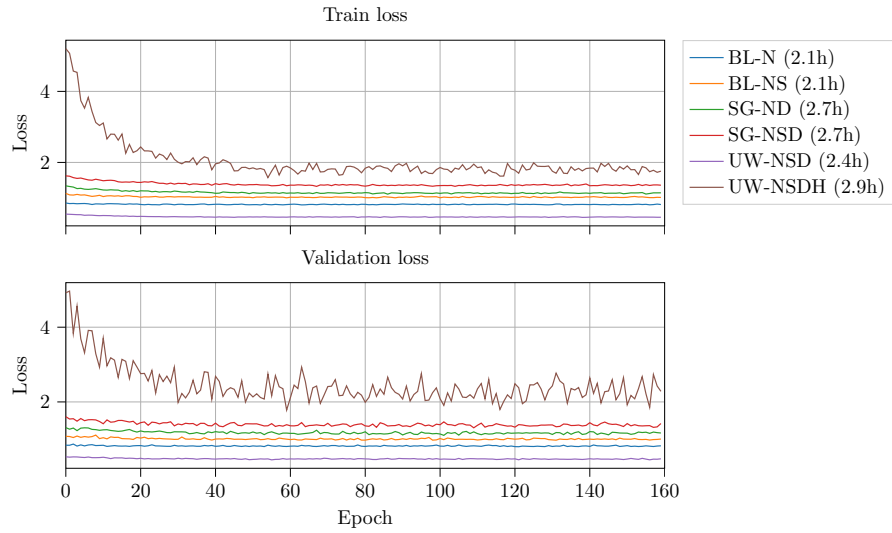

Figure S4: Train and validation loss of the models trained on the OSLO-COMET dataset from finetuning the entire architecture.

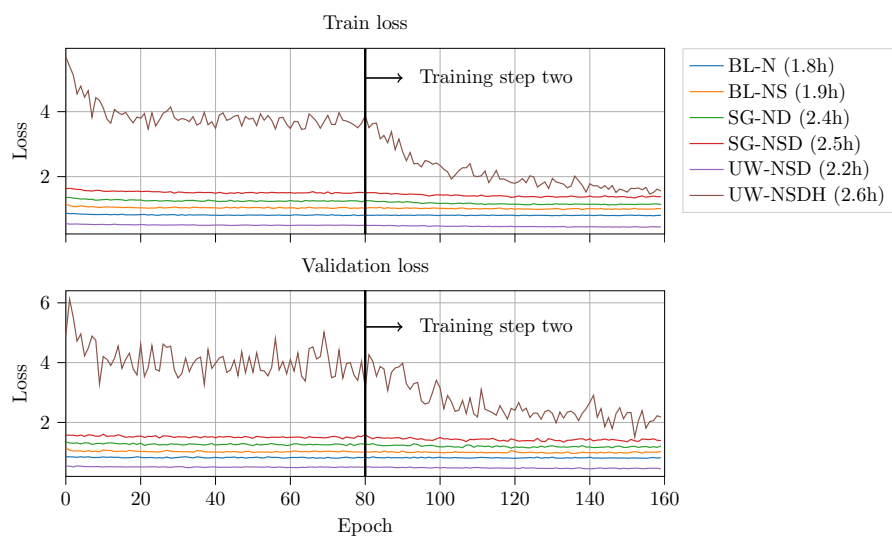

Figure S5: Train and validation loss of the models trained on the OSLO-COMET dataset from finetuning in two steps.

### 2.3 Adaptive loss weighting results

Figs. S6 - S13 show the evolution of the dynamic weight in the UW models for the studied cases.

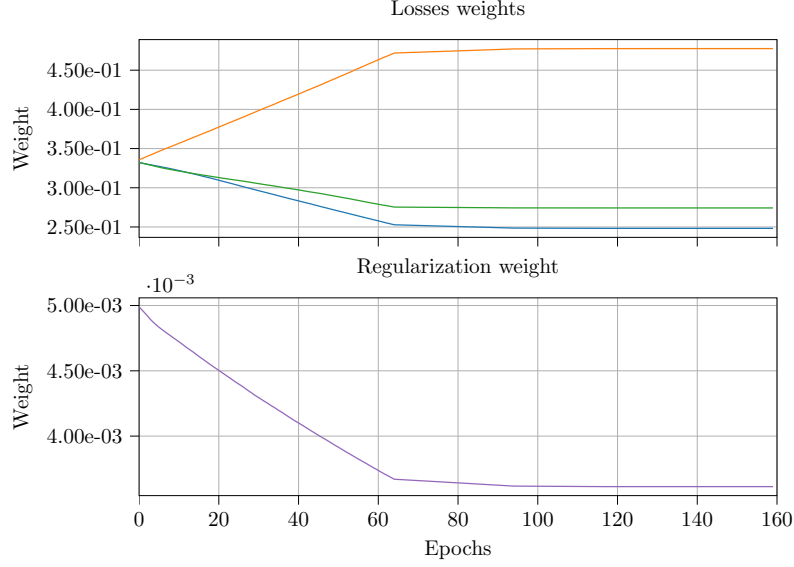

Figure S6: Loss weights of the model UW-NSD trained on the IXI dataset.

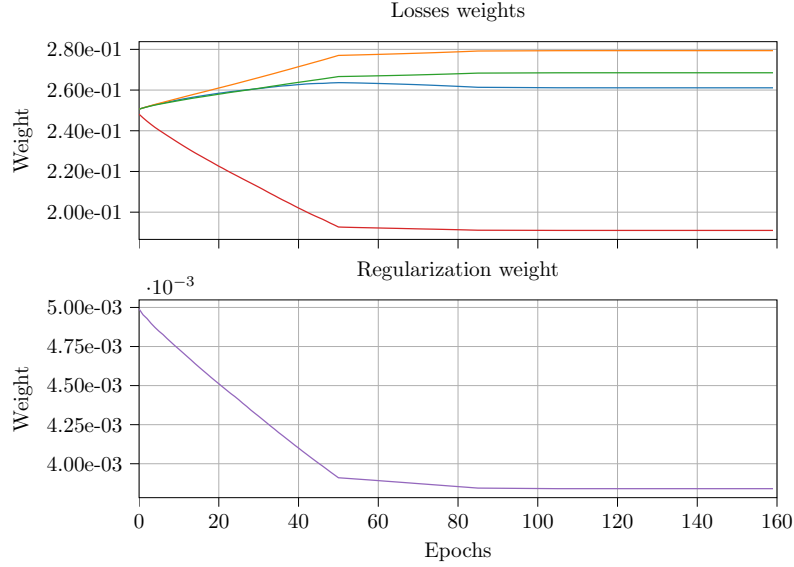

Figure S7: Loss weights of the model UW-NSDH trained on the IXI dataset.

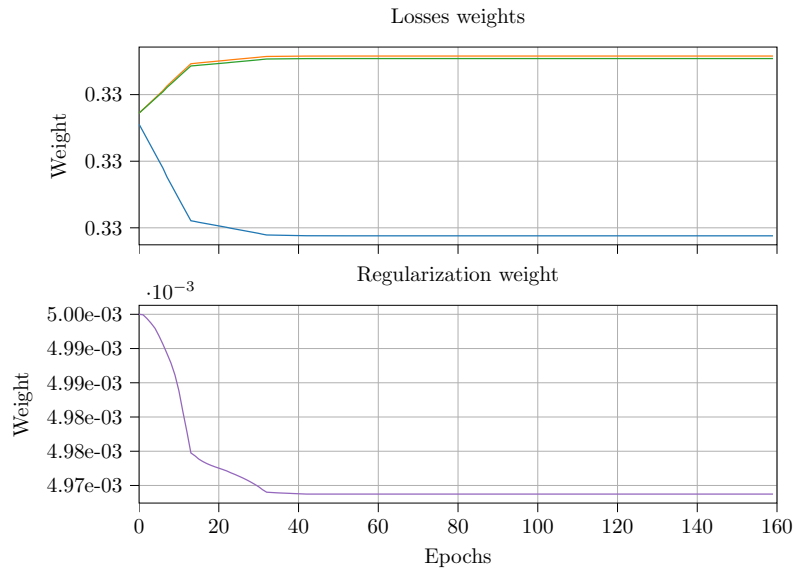

Figure S8: Loss weights of the model UW-NSD trained on the OSLO-COMET dataset.

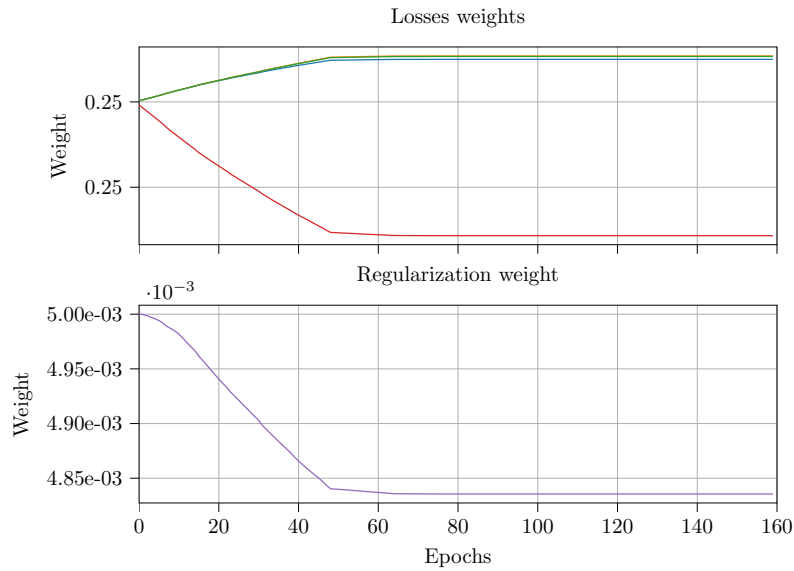

Figure S9: Loss weights of the model UW-NSDH trained on the OSLO-COMET dataset.

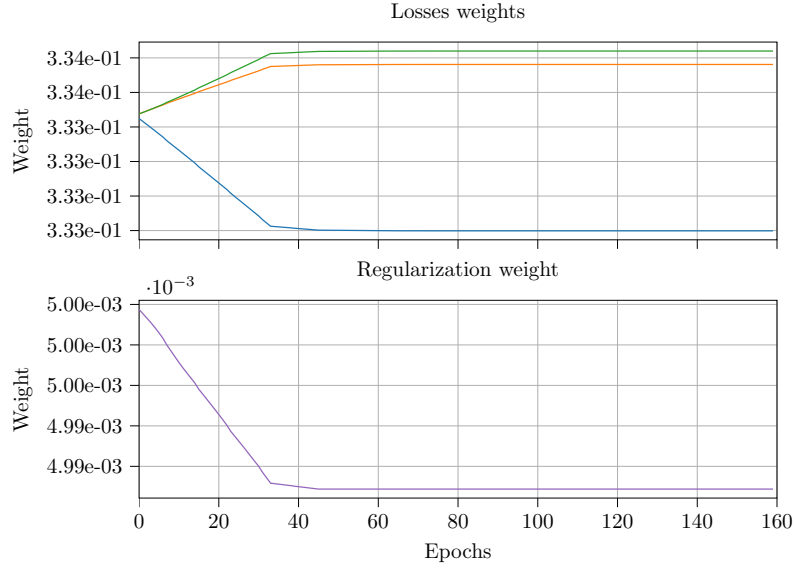

Figure S10: Loss weights of the model UW-NSD trained on the COEMT dataset from finetuning the entire architecture.

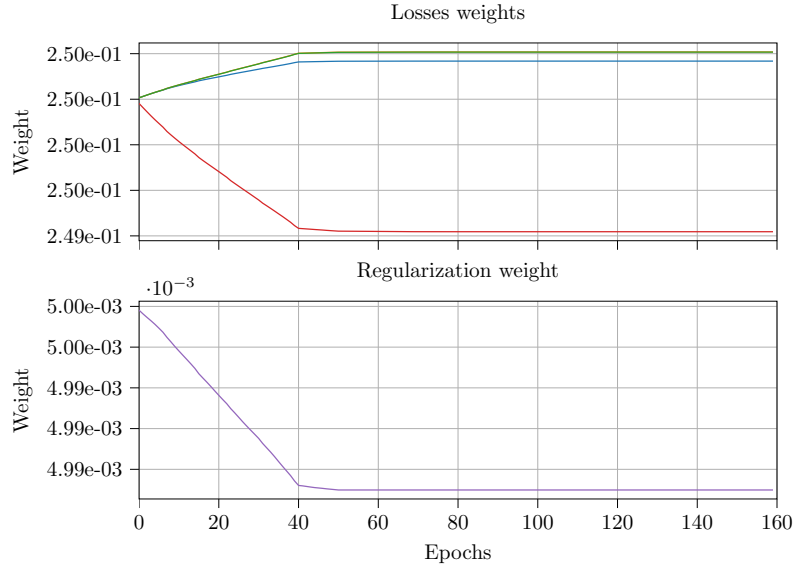

Figure S11: Loss weights of the model UW-NSDH trained on the COEMT dataset from finetuning the entire architecture.

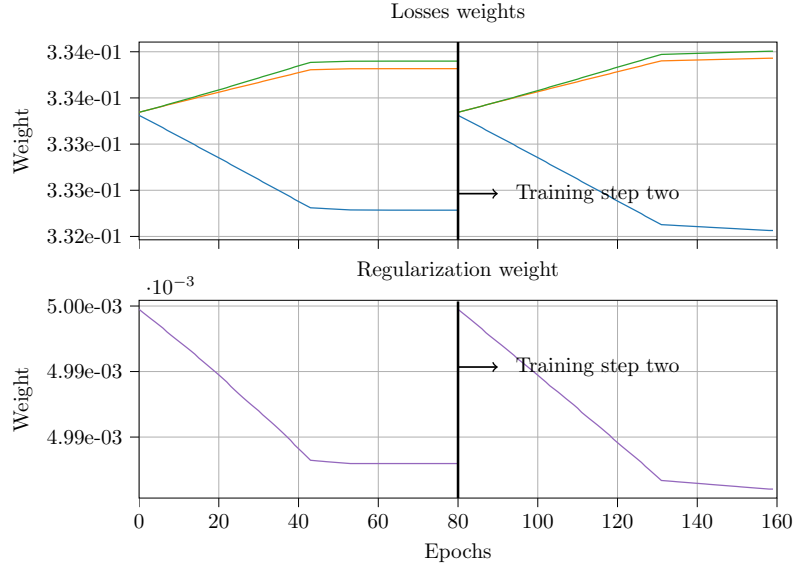

Figure S12: Loss weights of the model UW-NSD trained on the COEMT dataset from finetuning in two steps.

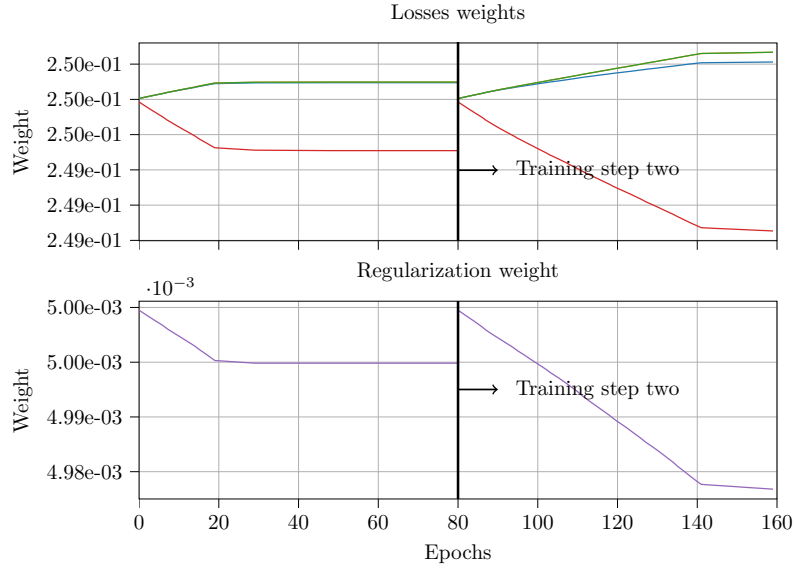

Figure S13: Loss weights of the model UW-NSDH trained on the COEMT dataset from finetuning in two steps.

## 2.4 Qualitative registration results

Examples of predictions on the IXI and OSLO-COMET test datasets.

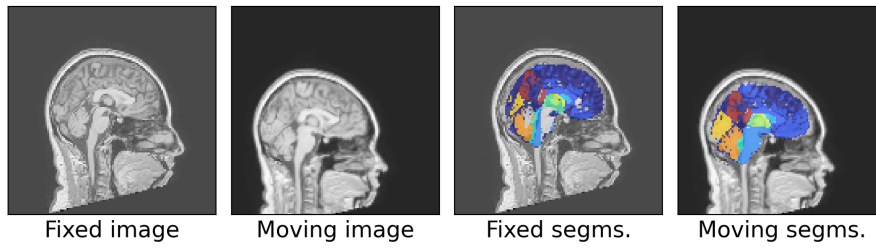

(a) Sample test image.

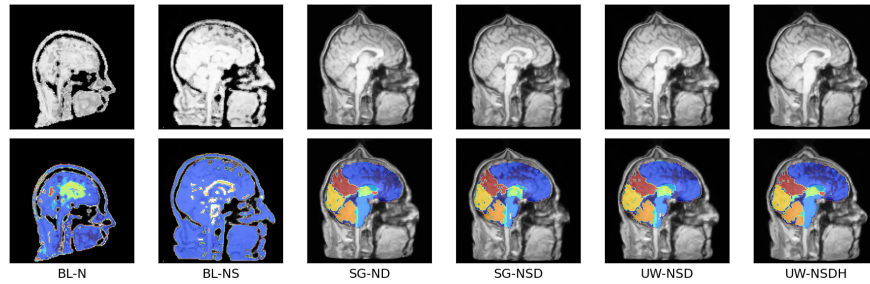

(b) Predictions of the evaluated models on the sample image.

Figure S14: Sample image of the IXI test set, and predictions of the models.

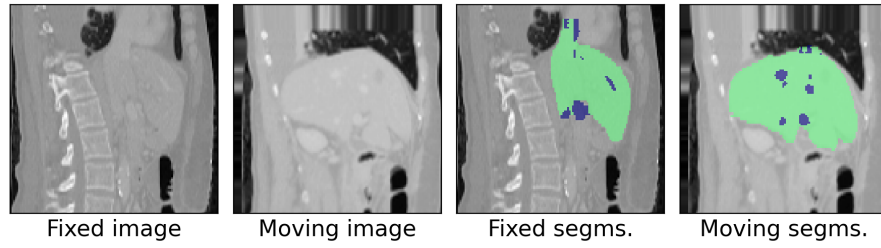

(a) Sample test image.

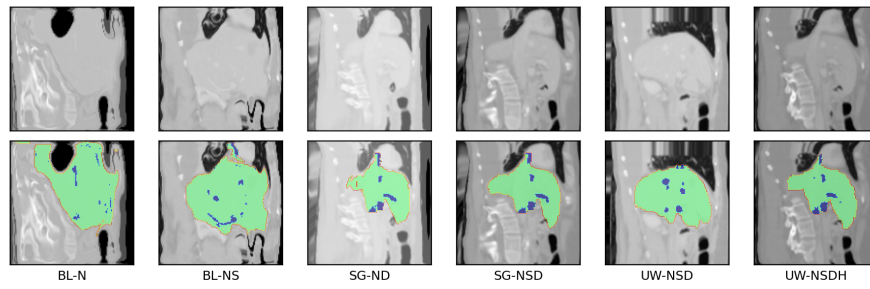

(b) Predictions of the models trained on the OSLO-COMET dataset.

Figure S15: Sample image of the OSLO-COMET test set, and predictions of the models trained on the OSLO-COMET dataset.

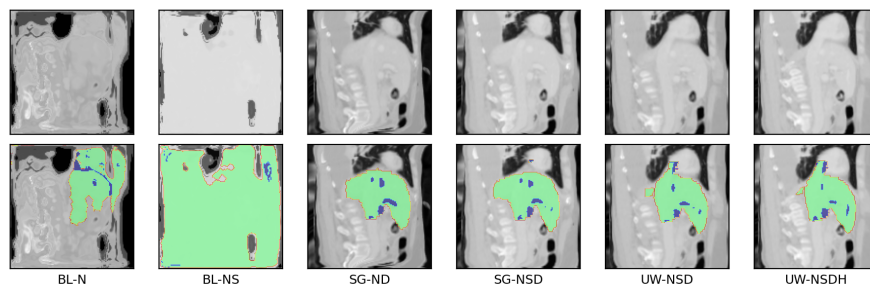

(a) Predictions of the models trained on the OSLO-COMET dataset from finetuning the entire architecture.

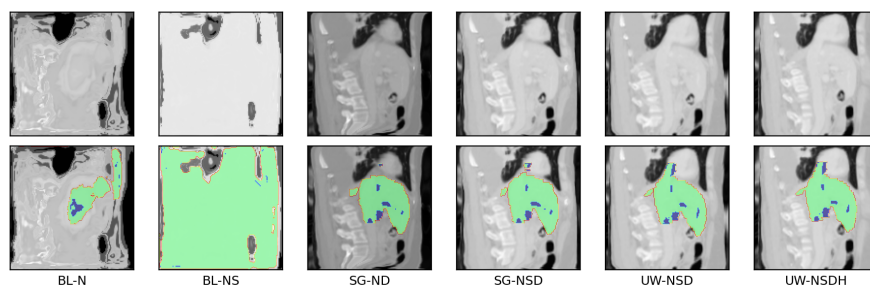

(b) Predictions of the models trained on the OSLO-COMET dataset from finetuning in two steps.

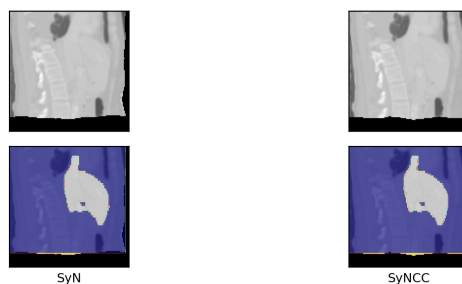

(c) Predictions of the SyN and SyNCC algorithms.

Figure S16: Predictions of the finetuned models and ANTs on the OSLO-COMET test set sample.
